# Supplementary material for: Energy Efficient Cloud Control and Pricing in Geographically Distributed Data Centers
Source: arXiv:1809.05853 source file (2018-09-16)
Supplement: Supplementary file 2 [file cv.tex]

% Jason R. Blevins - Curriculum Vitae
%
% Copyright (C) 2004-2011 Jason R. Blevins
%
% You may use use this document as a template to create your own CV
% and you may redistribute the source code freely.  No attribution is
% required in any resulting documents.  I do ask that you please leave
% this notice and the above URL in the source code if you choose to
% redistribute this file.

\documentclass[10pt,letterpaper]{article}

\usepackage{hyperref}
\usepackage{geometry}

% Fonts
\usepackage[T1]{fontenc}
\usepackage[urw-garamond]{mathdesign}

% Set your name here
\def\name{Jason R. Blevins}

% The following metadata will show up in the PDF properties
\hypersetup{
  colorlinks = true,
  urlcolor = black,
  pdfauthor = {\name},
  pdfkeywords = {economics, econometrics, industrial organization,
    applied microeconomics},
  pdftitle = {\name: Curriculum Vitae},
  pdfsubject = {Curriculum Vitae},
  pdfpagemode = UseNone
}

\geometry{
  body={6.5in, 9.0in},
  left=1.0in,
  top=1.0in
}

% Customize page headers
\pagestyle{myheadings}
\markright{\name}
\thispagestyle{empty}

% Custom section fonts
\usepackage{sectsty}
\sectionfont{\rmfamily\mdseries\Large}
\subsectionfont{\rmfamily\mdseries\itshape\large}

% Other possible font commands include:
% \ttfamily for teletype,
% \sffamily for sans serif,
% \bfseries for bold,
% \scshape for small caps,
% \normalsize, \large, \Large, \LARGE sizes.

% Don't indent paragraphs.
\setlength\parindent{0em}

% Make lists without bullets and compact spacing
\renewenvironment{itemize}{
  \begin{list}{}{
    \setlength{\leftmargin}{1.5em}
    \setlength{\itemsep}{0.25em}
    \setlength{\parskip}{0pt}
    \setlength{\parsep}{0.25em}
  }
}{
  \end{list}
}

\begin{document}

% Place name at left
{\huge \name}

% Alternatively, print name centered and bold:
%\centerline{\huge \bf \name}

\bigskip

\begin{minipage}[t]{0.5\textwidth}
  Department of Economics \\
  The Ohio State University \\
  410 Arps Hall \\
  1945 N High Street \\
  Columbus, OH 43210
\end{minipage}
\begin{minipage}[t]{0.5\textwidth}
  Phone: (614) 292-5588 \\
  Fax: (614) 292-3906 \\
  Office: 415 Arps Hall \\
  Email: \href{mailto:blevins.141@osu.edu}{blevins.141@osu.edu} \\
  Homepage: \href{http://jblevins.org/}{http://jblevins.org/}
\end{minipage}

\section*{Education}

\begin{itemize}
  \item Ph.D. Economics, Duke University, 2010.
    % Received May 16, 2010
    \begin{itemize}
    \item \textit{Dissertation:}
      Essays in Industrial Organization and Econometrics.
    \item \textit{Committee:}
      Han Hong (co-chair), Shakeeb Khan (co-chair),
      Paul Ellickson, and Andrew Sweeting.
    \end{itemize}
  \item M.A. Economics, Duke University, 2006.
    % Received May 14, 2006
  \item B.S. Applied Mathematics, \textit{Summa Cum Laude},
    North Carolina State University, 2004.
    % Received May 14, 2004
  \item Budapest Semesters in Mathematics, Fall 2002.
\end{itemize}

\section*{Employment}

\begin{itemize}
\item Assistant Professor, Department of Economics, The Ohio State University,
  July 2010--present.
\end{itemize}

% \subsection*{Duke University, Department of Economics}
%
% \begin{itemize}
% \item Research Assistant, Jacob Vigdor, Summer 2005--Summer 2006.
% \item Teaching Assistant, Ph.D. Microeconomic Analysis, Thomas Nechyba, Fall 2005.
% \item Teaching Assistant, Ph.D. Game Theory, Curtis Taylor, Spring 2006.
% \item Instructor, Microeconomics Qualifier Camp, Summer 2006.
% \item Research Assistant, Han Hong, Fall 2006--Spring 2007.
% \item Research Assistant, Aprajit Mahajan and Alessandro Tarozzi,
%   October--November 2006, March--June 2007.
% \item Research Assistant, Shakeeb Khan and Christopher Timmins,
%   March--June 2007.
% \item Teaching Assistant, Ph.D. Econometrics II, Shakeeb Khan,
%   Spring 2007.
% \item Research Assistant, Peter Arcidiacono, Patrick Bayer,
%   and Paul Ellickson, Fall 2007--Spring 2009.
% \item Research Assistant, Shakeeb Khan, Fall 2009--Spring 2010.
% \item Research Assistant, Aprajit Mahajan, July--September 2009.
% \end{itemize}

% \subsection*{North Carolina State University, Department of Mathematics}
%
% \begin{itemize}
% \item Research Assistant, Moody Chu and Robert Funderlic,
%   Spring 2003--Fall 2004.
% \item Mathematics Tutor, Academic Support Program for Student Athletes,
%   Summer 2001.
% \end{itemize}

% \subsection*{Colorado School of Mines,
%   Department of Mathematical and Computer Sciences}
%
% \begin{itemize}
% \item Research Assistant, Willy Hereman, Summer 2002.
% \end{itemize}

\section*{Fields of Research Interest}

Econometrics and Empirical Industrial Organization

\section*{Research}

\subsection*{Working Papers}

\begin{itemize}
\item Blevins, J.~R. (2011).
  \href{http://jblevins.org/research/panel}{Partial Identification and Inference in Binary Choice and Duration Panel Data Models}.
\item Blevins, J.~R. (2010).
  \href{http://jblevins.org/research/dcident}{Nonparametric Identification of Dynamic Games with Discrete and Continuous Choices}, \textit{under revision}.
\item Blevins, J.~R. and S.~Khan (2010).
  \href{http://jblevins.org/research/lnlls}{Local NLLS Estimation of Semiparametric Binary Choice Models}, \textit{under revision}.
\item Arcidiacono, P., P.~Bayer, J.~R. Blevins, P.~B. Ellickson (2010).
  \href{http://jblevins.org/research/abbe}{Estimation of Dynamic Discrete Choice Models in Continuous Time}, \textit{under revision}.
\item Blevins, J.~R. and S. Khan (2009).
  \href{http://jblevins.org/research/dfbr}{Distribution-Free Estimation of Heteroskedastic Binary Response Models in Stata}.
\item Blevins, J.~R. (2011).
  \href{http://jblevins.org/research/smcdmm}{Sequential Monte Carlo Methods for Estimating Dynamic Microeconomic Models},
  \textit{under review}.
\item Blevins, J.~R. (2008).
  \href{http://jblevins.org/research/seqgame}{Structural Estimation of Sequential Games of Complete Information}.
\end{itemize}

% \subsection*{Scientific Software}
%
% \begin{itemize}
% \item \href{http://jblevins.org/research/pdest}{PDESolutionTester},
%   A Mathematica program for the symbolic verification of exact solutions
%   of nonlinear partial differential equations,
%   with Jeff Heath and Willy Hereman (2002).
% \item \href{http://jblevins.org/research/dfbr}{DFBR},
%   A Stata program for distribution-free estimation of heteroskedastic
%   binary response models,
%   with Shakeeb Khan (2009).
% \end{itemize}

\subsection*{Other Publications}

\begin{itemize}

\item Blevins, J.~R. (2009).
  \href{http://jblevins.org/research/generic-list}{A Generic Linked List Implementation in Fortran 95}.
  \textit{ACM Fortran Forum} 28(3), 2--7.

\end{itemize}

\section*{Teaching}

\subsection*{The Ohio State University}

\begin{itemize}
\item \href{http://jblevins.org/courses/econ843f11/}{Research Topics in Microeconometrics} (Ph.D.),
  Fall 2011. % 5 credit hours
\item \href{http://jblevins.org/courses/econ741s11/}{General Linear Regression Analysis} (Ph.D.),
  Spring 2011. % 47 students, 5 credit hours
\item \href{http://jblevins.org/courses/econ444w11/}{Elementary Econometrics},
  Winter 2011. % 57 students, 5 credit hours
\end{itemize}

\subsection*{Duke University}

\begin{itemize}
\item \href{http://jblevins.org/courses/econ342s07/}{Econometrics II} (Ph.D.), Spring 2007, Teaching Assistant for Shakeeb Khan.
\item \href{http://jblevins.org/courses/qualcamp06/}{Microeconomics Qualifier Camp} (Ph.D.), Summer 2006, Instructor.
\item \href{http://jblevins.org/courses/econ302s06/}{Microeconomic Analysis II} (Ph.D.), Spring 2006, Teaching Assistant for Curtis Taylor.
\item \href{http://jblevins.org/courses/econ301f05/}{Microeconomic Analysis I} (Ph.D.), Fall 2005, Teaching Assistant for Thomas Nechyba.
\end{itemize}

\section*{Conference and Seminar Presentations}

\begin{itemize}

\item \href{http://jblevins.org/research/panel}{Partial Identification and Inference in Binary Choice and Duration
    Panel Data Models}

  \begin{itemize}
  \item Vanderbilt University, Department of Economics,
    September 15, 2011 (scheduled).
  \item University of Texas at Austin, Department of Economics,
    April 4, 2011.
  \item 20th Annual Meetings of the Midwest Econometrics Group,
    Washington University,
    October 2, 2010.
  \item University of Illinois at Urbana-Champaign, Department of Economics,
    February 16, 2010.
  \item University of Pittsburgh, Department of Economics,
    January 15, 2010.
  \item Triangle Econometrics Conference,
    Research Triangle Park, NC,
    December 4, 2009.
  \end{itemize}

\item \href{http://jblevins.org/research/dcident}{Nonparametric Identification of Dynamic Games with Discrete and Continuous Choices}

  \begin{itemize}
    \item 2011 Meetings of the Midwest Econometrics Group,
      University of Chicago Booth School of Business,
      October 7, 2011 (scheduled).
  \end{itemize}

\item \href{http://jblevins.org/research/abbe}{Estimation of Dynamic Discrete Choice Models in Continuous Time}

  \begin{itemize}
  \item Pennsylvania State University, Department of Economics,
    November 7, 2011 (scheduled).
  \item University of Western Ontario, Department of Economics,
    January 26, 2010.
  \item The Ohio State University, Department of Economics,
    January 21, 2010.
  \end{itemize}

\item \href{http://jblevins.org/research/smcdmm}{Sequential Monte Carlo Methods for Estimating Dynamic Microeconomic Models}

  \begin{itemize}
  \item University of Rochester, Simon Graduate School of Business,
    May 6, 2011.
  \item The Ohio State University,
    Department of Agricultural, Environmental, and Development Economics,
    April 21, 2011.
  \item ERID Conference on Identification Issues in Economics,
    Duke University, October 3, 2008.
  \end{itemize}

\end{itemize}

\section*{Professional Activities}

\begin{itemize}
\item Reviewer for
  \textit{Econometrica}, % 2011
  \textit{Economic Inquiry}, % 2008 (1)
  \textit{Journal of Business and Economic Statistics}, % 2009 (1)
  \textit{Journal of Computational Finance}, % 2010 (1)
  \textit{Journal of Econometrics}, % 2009 (1), 2011 (1)
  \textit{Scandinavian Journal of Statistics}, % 2009 (1)
  Cambridge University Press. % 2011
\item Departmental service:
  Faculty Recruiting Committee (2010-11, 2011-12),
  G.S. Maddala Prize Committee (2010-11).
\item Member, Econometric Society, 2006--Present.
\item Member, American Economic Association, 2010--Present.
\end{itemize}

\section*{Advising}

\begin{itemize}
\item Ph.D. Students (secondary advisor):
  Chih-Sheng Hsieh (Ph.D. candidate), % candidacy exam, 2011
  Fei Jin (Ph.D. candidate),          % candidacy exam, 2011
  Seonghoon Kim (Ph.D. candidate).    % candidacy exam, 2011

\item Undergraduate Students:
  Erik Lauritzen (2011).
\end{itemize}

\section*{Honors, Awards, \& Fellowships}

\begin{itemize}
\item Summer Research Fellowship, Duke University, 2007, 2008.
\item Institute on Computational Economics Fellow, University of Chicago, 2006.
\item Outstanding Teaching Assistant Award, Duke University, 2006.
\item Undergraduate Research Award, North Carolina State University, 2004.
% \item Omicron Delta Epsilon, International Economics Honor Society, 2004.
\item Phi Beta Kappa, Zeta of North Carolina, 2003.
% \item Pi Mu Epsilon, National Mathematics Honor Society, 2003.
\item NSF Research Experiences for Undergraduates, Colorado School of Mines, 2002.
% \item Phi Kappa Phi, 2002.
% \item Golden Key International Honour Society, 2002.
% \item Dean's List, North Carolina State University, 2000--2004.
\end{itemize}

\section*{Conferences and Workshops Attended}

\begin{itemize}
\item 2011 Meetings of the Midwest Econometrics Group,
  University of Chicago Booth School of Business,
  October 6-7, 2011 (scheduled).
\item North American Summer Meetings of the Econometric Society,
  Washington University,
  June 9--12, 2011.
\item AEA/ASSA Annual Meetings,
  Denver, CO, January 6--10, 2011.
\item 20th Annual Meetings of the Midwest Econometrics Group,
  Washington University,
  October 1--2, 2010.
\item AEA/ASSA Annual Meetings,
  Atlanta, GA, January 3--5, 2010.
\item Triangle Econometrics Conference,
  Research Triangle Park, NC,
  December 4, 2009.
\item Cowles Foundation Conference, Applications of Structural Microeconomics,
  Yale University,
  June 24--25, 2009.
\item ERID Conference on Identification,
  Duke University,
  October 3--4, 2008.
\item North American Summer Meetings of the Econometric Society,
  Duke University,
  June 21--24, 2007.
\item Institute on Computational Economics,
  Argonne National Laboratory,
  July 17--21, 2006.
\item SIAM Conference on Applied Linear Algebra,
  The College of William \& Mary,
  July 15--19, 2003.
\end{itemize}

\section*{Miscellaneous}

\begin{itemize}
\item \textit{Security Clearance:} Special Sworn Status, U.S. Census Bureau.
\end{itemize}

\medskip

% Footer
\begin{center}
  \begin{small}
    Last updated: \today
  \end{small}
\end{center}

\end{document}
