# Supplementary material for: Energy Efficient Cloud Control and Pricing in Geographically Distributed Data Centers
Source: arXiv:1809.05853 source file (2018-09-16)
Supplement: Supplementary file 3 [file footer.tex]

\medskip

% Footer
\begin{center}
  \begin{small}
    Curriculum vit\ae\ last updated: \today
  \end{small}
\end{center}
