# Supplementary material for: Energy Efficient Cloud Control and Pricing in Geographically Distributed Data Centers
Source: arXiv:1809.05853 source file (2018-09-16)
Supplement: Supplementary file 4 [file pro_activities.tex]

\section*{Professional activities}

\subsection*{Talks}
\begin{itemize}
  \item OpenStack: build a cloud! \href{http://webcampzg.org}{WebCampZG 2012}, Zagreb, \
  Croatia; 24 November, 2012. %(\href{http://webcampzg.org/drazen-lucanin-openstack-izgradite-svoj-oblak/}{slides})
\end{itemize}

\subsection*{Conferences attended}
\begin{itemize}
  \item \href{https://conc.at/}{.concat() 2015}, Salzburg, Austria; 7 March, 2015.
  \item \href{https://ep2014.europython.eu/}{EuroPython 2014}, Berlin, Germany; 21-27 July, 2014.
  \item \href{http://codefront.io/}{Codefront.io 2014}, Linz, Austria; 10 May, 2014.
  \item \href{http://linz.kod.io/}{Kod.io 2014}, Linz, Austria; 1 March, 2014.
  \item \href{http://13.rupy.eu/}{RuPy 2013}, Budapest, Hungary; 11-13 October, 2013.
  \item \href{https://ep2013.europython.eu/}{EuroPython 2013}, Florence, Italy; 1-7 July, 2013.
  \item \href{http://12.rupy.eu}{RuPy 2012}, Brno, Czech Republic; 16-18 November, 2012.
  \item \href{https://ep2012.europython.eu/}{EuroPython 2012}, Florence, Italy; 2-8 July, 2012.
\end{itemize}
