# Supplementary material for: Energy Efficient Cloud Control and Pricing in Geographically Distributed Data Centers
Source: arXiv:1809.05853 source file (2018-09-16)
Supplement: Supplementary file 6 [file Drazen_Lucanin-CV.tex]

\input{meta/header}

\begin{document}

\toggletrue{full}

% contact
\input{sections/contact}

% education
\input{sections/education/basic}
\input{sections/education/extra}
\input{sections/education/abroad}

% employment
\input{sections/employment/basic}
\input{sections/employment/extra}
\input{sections/employment/voluntary}

% research
\input{sections/research/all}

\input{sections/awards}

\input{sections/skills/all}

\input{meta/footer}

\end{document}
