# Supplementary material for: Energy Efficient Cloud Control and Pricing in Geographically Distributed Data Centers
Source: arXiv:1809.05853 source file (2018-09-16)
Supplement: Supplementary file 7 [file header.tex]

%
% Drazen Lucanin's CV.
%
% Original LaTeX template:
%
% Jason R. Blevins - Curriculum Vitae
%
% Copyright (C) 2004-2010 Jason R. Blevins
%
% You may use use this document as a template to create your own CV
% and you may redistribute the source code freely.  No attribution is
% required in any resulting documents.  I do ask that you please leave
% this notice and the above URL in the source code if you choose to
% redistribute this file.

\documentclass[10pt,letterpaper]{article}

\makeatletter
\@ifpackageloaded{tex4ht}{\def\iftex4ht{\iftrue}}
                         {\def\iftex4ht{\iffalse}}
\makeatother

\usepackage{etoolbox}
\usepackage{hyperref}
\usepackage{geometry}
\usepackage{longtable}
%\usepackage{tablefootnote}
%\usepackage{tabularx}
%\usepackage[monochrome]{color}

% Fonts
\usepackage[T1]{fontenc}
\usepackage[utf8]{inputenc}
%\usepackage[urw-garamond]{mathdesign}

\iftex4ht
\else
%\usepackage[urw-garamond]{mathdesign}
\usepackage[adobe-utopia]{mathdesign} 
\fi

\usepackage[super]{nth}

% Set your name here
\def\name{Dražen Lučanin}

%\def\link-color{blue}
%\def\linkcolor{red}
\def\linkcolor{black}

\hypersetup{
% The following metadata will show up in the PDF properties
  pdfauthor = {\name},
  pdfkeywords = {computer science, artificial intelligence,
  machine learning, pattern recognition},
  pdftitle = {\name: Curriculum Vitae},
  pdfsubject = {Curriculum Vitae},
  pdfpagemode = UseNone,
% PDF design	
	colorlinks=true, linkcolor=\linkcolor ,  anchorcolor=\linkcolor ,
	citecolor=\linkcolor , filecolor=\linkcolor , menucolor=\linkcolor ,
	urlcolor=\linkcolor
}
\geometry{
  body={6.5in, 9.0in},
  left=1.0in,
  top=1.0in
}

% Customize page headers
\pagestyle{myheadings}
\markright{\name\ -- Curriculum Vit\ae}
\thispagestyle{empty}

% Custom section fonts
\usepackage{sectsty}
\sectionfont{\rmfamily\mdseries\Large}
\subsectionfont{\rmfamily\mdseries\itshape\large}

% Other possible font commands include:
% \ttfamily for teletype,
% \sffamily for sans serif,
% \bfseries for bold,
% \scshape for small caps,
% \normalsize, \large, \Large, \LARGE sizes.

% Don't indent paragraphs.
\setlength\parindent{0em}

% Make lists without bullets and compact spacing
\renewenvironment{itemize}{
  \begin{list}{}{
    \setlength{\leftmargin}{1.5em}
    \setlength{\itemsep}{0.25em}
    \setlength{\parskip}{0pt}
    \setlength{\parsep}{0.25em}
  }
}{
  \end{list}
}

\newtoggle{full}
\newtoggle{publicationURLs}
