# Supplementary material for: Energy Efficient Cloud Control and Pricing in Geographically Distributed Data Centers
Source: arXiv:1809.05853 source file (2018-09-16)
Supplement: Supplementary file 8 [file abroad.tex]

\subsection*{Education abroad}
\label{sec:education.abroad}
Two times participant of the Erasmus student exchange program:
\begin{itemize}
  \item \underline{2011}\\
  One semester at the University of Vienna during MS\\
  Master's thesis + courses
  
  \item \underline{2009}\\
  One semester at the University of Vienna during BS\\
  Bachelor's thesis + courses
	
	
  \item \textbf{Note:} Passed several courses (15 ECTS points in 2009 and 6 ECTS points in 2011) in parallel in the field of computer science at the Vienna University of Technology.
\end{itemize}

Participated in a distributed course - a programming project (Visual Architecture, see section \nameref{sec:projects}) in a multicultural team of people from Africa, Asia and Europe. Was officially enrolled at Mälardalen University, Sweden.
\begin{itemize}
  \item \href{http://www.fer.hr/rasip/dsd}{Distributed Software Development}\\
	University of Zagreb, Croatia and Mälardalen University, Sweden
\end{itemize}
