# Supplementary material for: Energy Efficient Cloud Control and Pricing in Geographically Distributed Data Centers
Source: arXiv:1809.05853 source file (2018-09-16)
Supplement: Supplementary file 9 [file extra.tex]

\begin{itemize}
  \item \underline{2002 - 2006}\\
  5th Gymnasium (focus: mathematics)\footnotemark\\
  Zagreb
  \footnotetext{
	Grade average: 5\\
	Graduation thesis: A program for solving linear equation systems using Cramer's rule.\\
	Mentor: Prof. Mate Vulić  
  }
  
  \item \underline{1994 - 2002}\\
  Primary School\\
  Zagreb
\end{itemize}
