# Supplementary material for: Energy Efficient Cloud Control and Pricing in Geographically Distributed Data Centers
Source: arXiv:1809.05853 source file (2018-09-16)
Supplement: Supplementary file 10 [file extra.tex]

\begin{itemize}
	\item \underline{June - July 2008}\\
	Part-time worker for the digitalization of a cadastral raster map in AutoCAD\\
	CADCOM d.o.o.
\end{itemize}
