# Supplementary material for: Energy Efficient Cloud Control and Pricing in Geographically Distributed Data Centers
Source: arXiv:1809.05853 source file (2018-09-16)
Supplement: Supplementary file 11 [file voluntary.tex]

\subsection*{Voluntary work}
\label{sec:employment.voluntary}
\begin{itemize}
  
  	\item \underline{23 - 30 July 2012}\\
	\href{http://s3.sci.hr/organizers.html#drazen}{School organiser}\\
	\href{http://s3.sci.hr/}{Višnjan Summer School of Science}
  
  	\item \underline{18 - 25 July 2011}\\
	\href{http://s3.sci.hr/programS32011.html#p3}{Automatic speech recognition} project leader\\
	\href{http://s3.sci.hr/}{Višnjan Summer School of Science}
  
	\item \underline{\nth{30} July - \nth{6} August 2010}\\
	\href{http://s3.sci.hr/programS32010.html#p1}{Machine Learning Algorithms for Face Recognition} project leader\\
	\href{http://s3.sci.hr/}{Višnjan Summer School of Science}
		
	 \item \underline{17 - 25 July 2010}\\
	 Porto Rico team guide\\
	 \href{http://ipho2010.hfd.hr/}{41st International Physics Olympiad in Zagreb}
	
	\item \underline{2007 - 2008}\\
	Member of the \href{http://www.fotokset.org/}{Photography Section of KSET}, FER student club
\end{itemize}
