# Supplementary material for: Energy Efficient Cloud Control and Pricing in Geographically Distributed Data Centers
Source: arXiv:1809.05853 source file (2018-09-16)
Supplement: Supplementary file 12 [file all.tex]

\section*{Research}
\label{sec:research}

\input{sections/research/interests}

\input{sections/research/projects}

\input{sections/research/publications}

\input{sections/research/activities}
