# Supplementary material for: Energy Efficient Cloud Control and Pricing in Geographically Distributed Data Centers
Source: arXiv:1809.05853 source file (2018-09-16)
Supplement: Supplementary file 13 [file interests.tex]

\subsection*{Research interests}
\begin{itemize}
  \item Large-scale distributed computing (parallel, cloud and P2P computing)
  \item Artificial intelligence (pattern recognition, machine learning)
  \item Modern GUIs (visual programming, advanced human-computer interaction)
  \item Open source (the ``bazaar'' development process, Ubuntu GNU/Linux)
\end{itemize}
