# Supplementary material for: Energy Efficient Cloud Control and Pricing in Geographically Distributed Data Centers
Source: arXiv:1809.05853 source file (2018-09-16)
Supplement: Supplementary file 16 [file all.tex]

\section*{Skills}

\subsection*{Foreign Languages}
\begin{itemize}
	\item English, fluent in speech and writing.\\
	\underline{2005} - Passed the Cambridge Level 1 Certificate in English (ESOL) with grade A.\\
	Studied it from early childhood. Worked and communicated in it with many native speakers.\\
	Certified level: B2. Self-assessment: C1 or higher.

	\item German\\
	Lived in Austria for 4 years.\\
	Certified level: B2

	\item Italian\\
	Certified level: A2
\end{itemize}

\subsection*{Professional skills}
\begin{itemize}

	\item Programming languages\\
	Most at home in: Python, Javascript\\
	Did projects in: Java, C\#, C, C++, Objective-C, \LaTeX.\\
	Some knowledge of: PHP, Pascal.

	\item Design\\
	Did work in HTML/CSS, Sass, Adobe Photoshop and InDesign.

	\item Operating Systems\\
	Proficient user of \emph{Linux}, OS X \& Windows.\\
	Done programming and other advanced tasks in all three.

	\item Specialized software\\
	Basic usage of Matlab, Mathematica, Adobe Flash and Photoshop, AutoCAD.

	\item Version control systems\\
	Bazaar, GIT, SVN.

	\item IDEs\\
	Emacs, Eclipse (\emph{PyDev}, JDT, CDT, TeXlipse), Visual Studio, Xcode, Qt Creator.

	\item System administration\\
	Experience in Linux server management, OpenStack deployment and usage, MySQL, PHP, Wordpress.

	\item Distributed development\\
	Active in open source development. Developer in two internationally\
        distributed software development\
	projects -- AMASL\ %(see section \nameref{sec:employment})\
	\& Visual Architecture. %(see section \nameref{sec:education.abroad}).

\end{itemize}

\subsection*{Other skills \& hobbies}
\begin{itemize}
	\item Guitar playing\\
	Finished two grades of classical music school, a private course and the \href{http://www.rock-akademija.hr/}{Rock Academy}.\\
	Played in several demo rock bands.

	\item Photography\\
	Finished two optional courses at the University of Zagreb and\
        was a member of the Photography Section of KSET.\ % (see section \nameref{sec:employment.voluntary}).
        Experience in both analog and digital photography.

	\item Drawing \& animation\\
	Author of the Epic Adventure web comic (see section \nameref{sec:projects}). Also interested in animation (done several amateur animations in Adobe Flash and in stop motion).

	\item Sports\\
	Trained many sports through life (tennis, fencing, rowing, sailing, skiing, kung-fu\dots) Always active. Currently recreationally doing cycling, swimming, hiking \& skiing.

	\item Literature\\
	Fan of classical literature, fantasy \& SF.

	%\item šuškanje
\end{itemize}

\section*{Programming projects}
\label{sec:projects}
\begin{itemize}
  	\item \href{https://launchpad.net/philharmonic}{Philharmonic}\\
  	An OpenStack scheduler written in Python\
  	that pauses virtual machines when electricity prices \
  	are predicted to be high in real-time pricing systems.\
  	Results published in a scientific paper\
  	(see section \nameref{sec:research}).
  	%Results pending review in a scientific paper.

  	\item \href{http://lis.irb.hr/foc/}{FOC}\\
  	A Python data extractor (part of a larger framework for forecasting\
  	financial crises) that fetches data from the\
  	\href{http://data.worldbank.org/developers}{World Bank's API} and\
  	\href{http://www.chidalgo.com/data.html}{C. Hidalgo's RCA indicators},\
  	couples it with the\
  	\href{http://www.imf.org/external/pubs/cat/longres.cfm?sk=26015.0}{IMF's crisis database}\
  	and formats it in machine-learning-friendly formats (for\
  	\href{http://rapid-i.com/content/view/181/190/}{Rapidminer} or\
  	\href{http://dms.irb.hr/}{subgroup discovery}). Caching to MongoDB.\
  	A Django web application built by \href{http://www.irb.hr/Ljudi/Matija-Piskorec}{M. Piškorec}\
  	on top of the extractor is available at \href{http://lis.irb.hr/foc/}{lis.irb.hr/foc} to\
  	illustrate its functionality. Results published in a scientific paper\
  	(see section \nameref{sec:research}).

	\item \href{https://launchpad.net/ogre-procedural-scene-generation}{libprocedural}\\
	A Python/C++ library for procedural scene generation in the Ogre 3D graphical engine. The library can be used through vIDE (see bellow). Basis for a master's thesis (see section \nameref{sec:education}).

	\item \href{https://launchpad.net/vide}{vIDE}\\
	A visual programming language environment built as an Eclipse IDE extension. Basis for a scientific paper (see section \nameref{sec:research}).

	\item Croatian Digit and Spelling Speech Recogniser\\
	A speech recognition system utilizing the CMU Pocketsphynx toolkit trained on a database of spelling and digit utterances in Croatian. Basis for a scientific paper (see section \nameref{sec:research}).

	\item \href{https://launchpad.net/robodj}{RoboDJ}\\
	A voting-architecture system for dynamically defining the playlist of a media player. Awarded best student program of 2010 at the Faculty of Electrical Engineering and Computing.

	\item \href{http://www.univie.ac.at/AMASL}{AMASL} Videochat\\
	A professional multimedia communication system for elderly people, created in a distributed environment with programmers from Austria, Netherlands and Croatia for the acclaimed AMASL project (see section \nameref{sec:employment}). Development of the video-conferencing module.

	\item \href{http://www.epska.org}{Epic Adventure}\\
	A fantasy web comic\\
	Content author, web page developer and designer

	\item \href{http://www.fer.hr/rasip/dsd/projects/visual_architecture}{Visual Architecture}\\
	An Eclipse IDE extension for visually editing computer architecture\
        diagrams and a coding \& debugging for an assembly language where\
        execution can be monitored through highlighting of certain elements\
        on the diagram. Developed as part of the Distributed Software
        Development course. %(see section \nameref{sec:education.abroad}).
	Project leader.

	\item Face Recogniser\\
	A face recognition program using PCA, Haar's feature extraction\
        \& SVM classification. Done as part of the Pattern Recognition course\
        (maximum points received). Was a mentor during a similar project at the\
        Višnjan Summer School of Science.\
        % (see section \nameref{sec:employment.voluntary}).

	\item Music Genre Recogniser\\
	A music genre recognition program using MFCC feature extraction \& SVM classification. Done as part of the Machine Learning course (maximum points received).

	\item C-like Programming Language Compiler\\
	A compiler for a language similar to C. Done as part of the Compiler Design course. Project got the most points per team-member in class.
	Team leader.

\end{itemize}
